# Supplementary material for: NeuroDAVIS: A neural network model for data visualization
Source: arXiv:2304.01222 ancillary file (2023-04-01)
Supplement: Supplementary file 1 [file NeuroDAVIS_Supplementary.pdf]

# NeuroDAVIS: A neural network model for data visualization

Supplementary Material

Chayan Maitra<sup>1</sup>   Dibyendu B. Seal<sup>2</sup>   Rajat K. De<sup>1\*</sup>

<sup>1</sup>Machine intelligence Unit, Indian Statistical Institute, Kolkata, 203 Barrackpore Trunk Road,  
Kolkata 700108, India.

<sup>2</sup>Tatras Data Services Pvt. Ltd., E64, Vasant Marg, Vasant Vihar, New Delhi 110057, India.

\*Corresponding author  
`rajat@isical.ac.in`

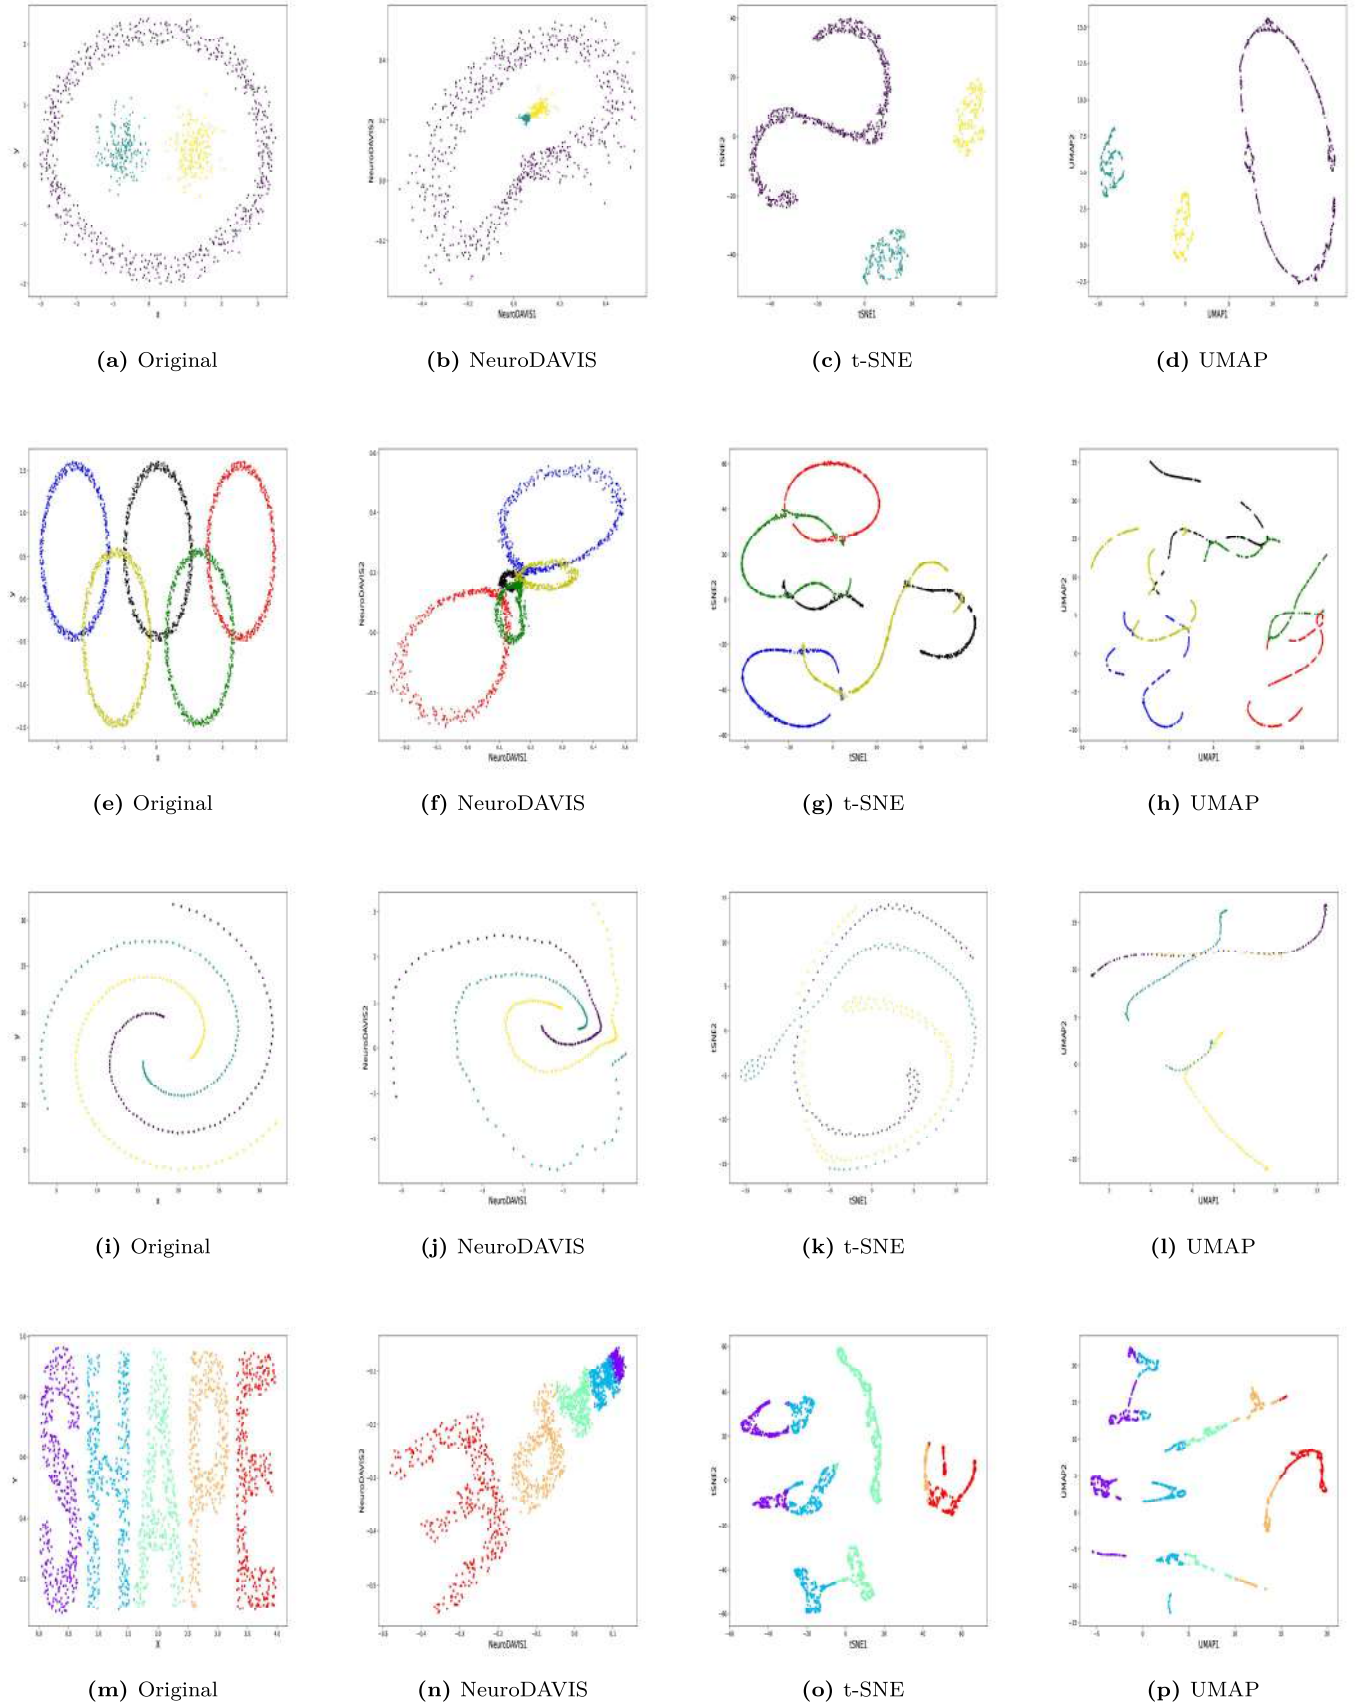

**Figure S1:** The original distributions and the embeddings produced by NeuroDAVIS, t-SNE and UMAP after a nine-dimensional transformation ( $x + y$ ,  $x - y$ ,  $xy$ ,  $x^2$ ,  $y^2$ ,  $x^2y$ ,  $xy^2$ ,  $x^3$ ,  $y^3$ ) of Elliptic Ring ((a)-(d)), Olympic ((e)-(h)), Spiral ((i)-(l)) and Shape ((m)-(p)) datasets.

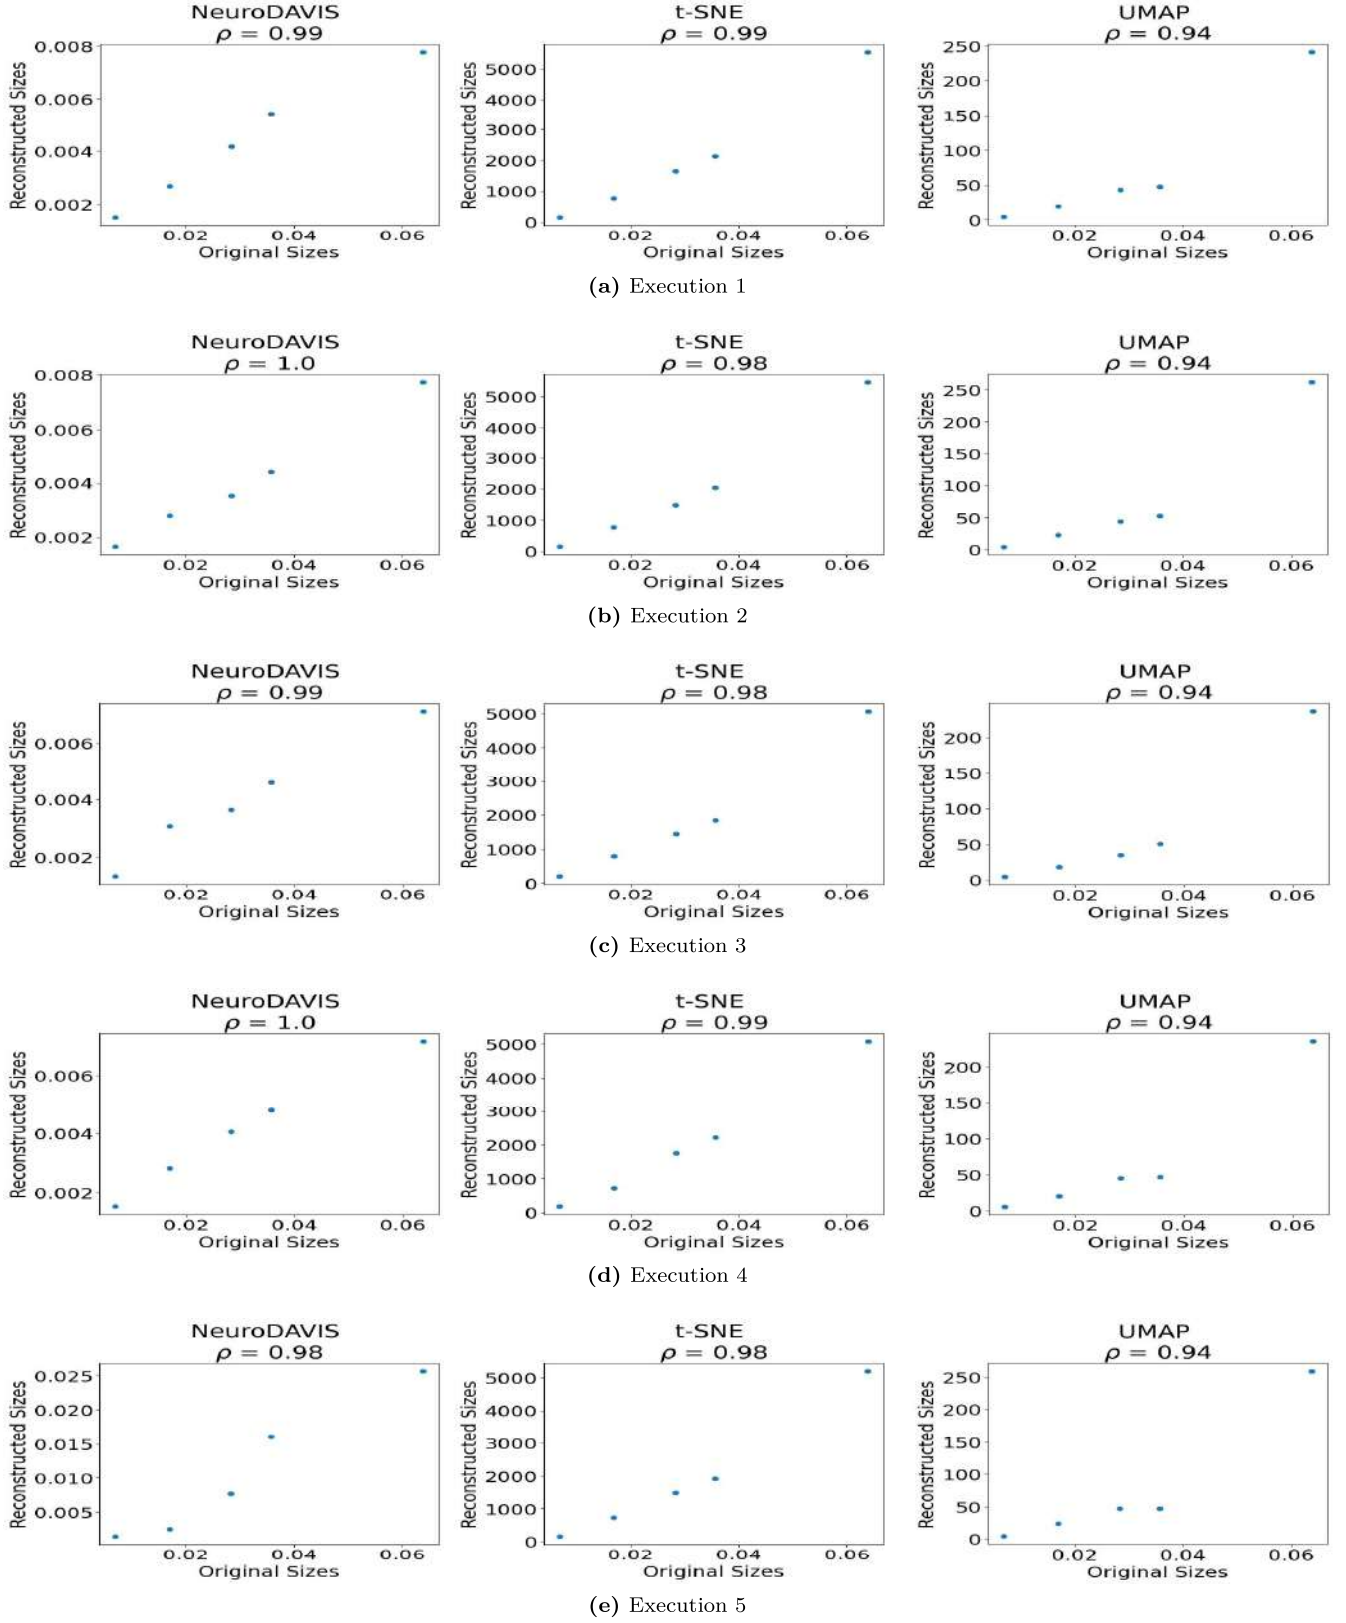

**Figure S2:** Preservation of cluster sizes by NeuroDAVIS, t-SNE and UMAP in World Map dataset.  $\rho$  is the Pearson correlation coefficient. Higher the  $\rho$  value, better is the preservation.

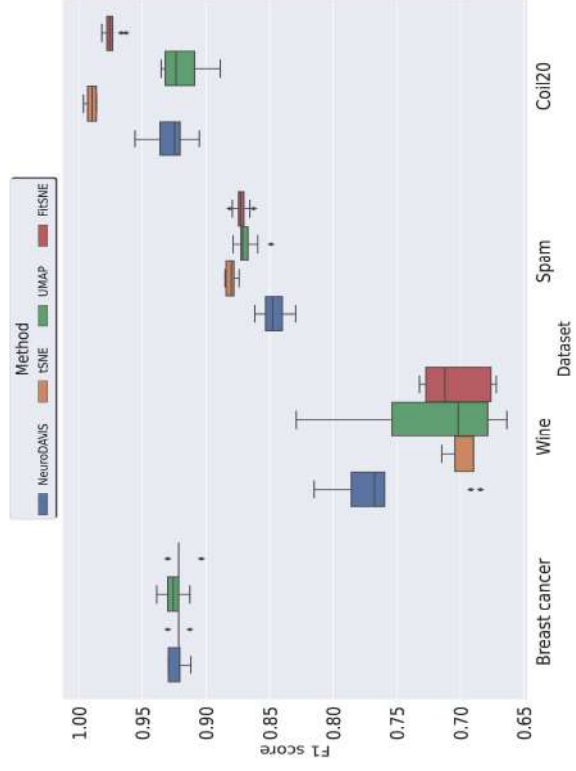

(a) Accuracy (k-nn)

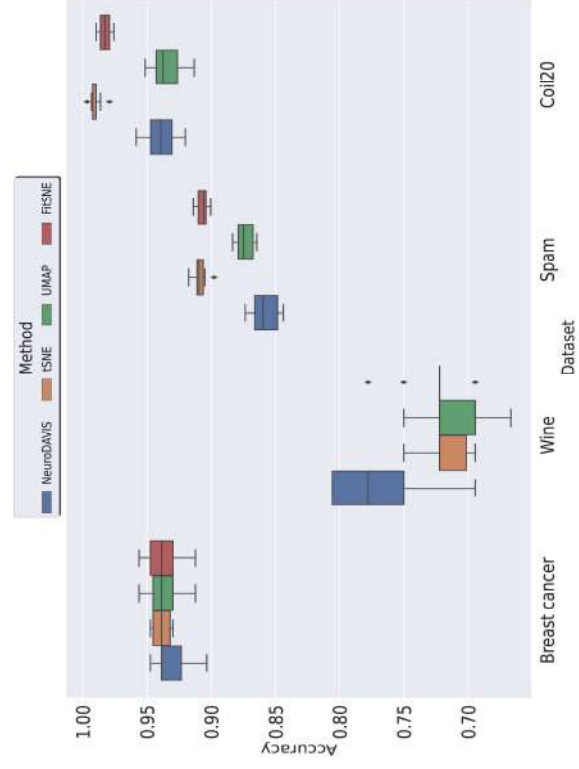

(c) Accuracy (RF)

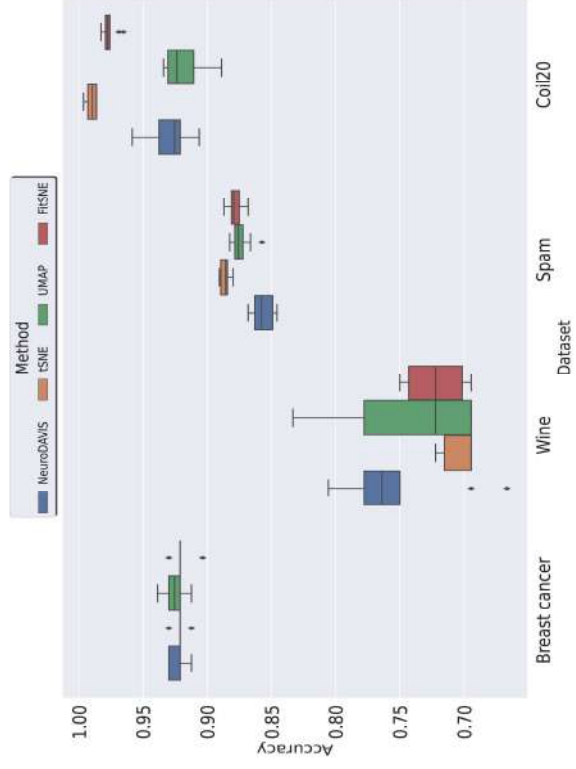

(b) F1-score (k-nn)

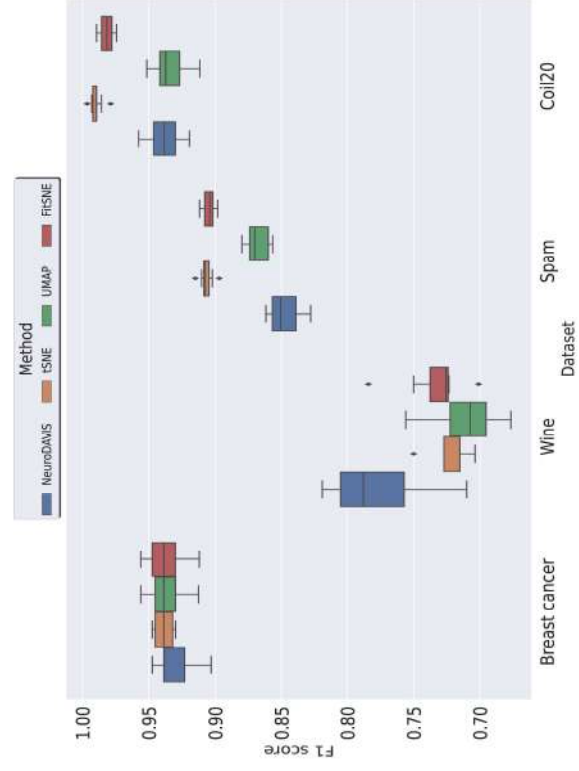

(d) F1-score (RF)

**Figure S3:** (a) and (b) show performance of k-nn classifier on NeuroDAVIS, t-SNE, UMAP and Fit-SNE-generated embeddings of Breast cancer, Wine, Spam and Coil20 datasets, in terms of Accuracy and F1-scores respectively, (c) and (d) show performance of random forest (RF) classifier on NeuroDAVIS, t-SNE, UMAP and Fit-SNE-generated embeddings of Breast cancer, Wine, Spam and Coil20 datasets, in terms of Accuracy and F1-scores respectively.

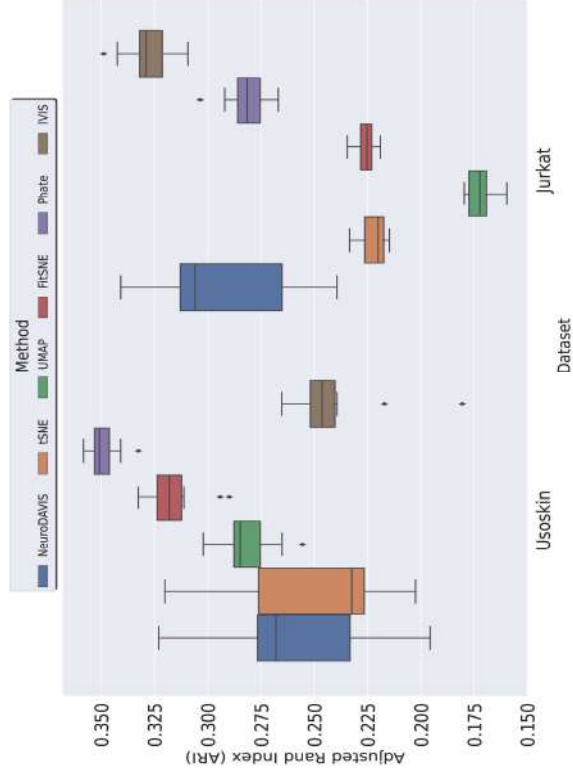

(a) Adjusted Rand Index (ARI) (k-means)

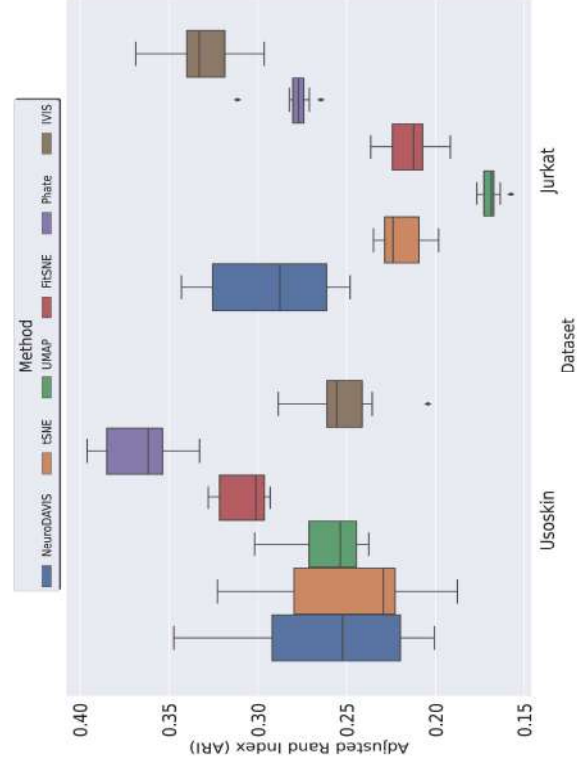

(c) Adjusted Rand Index (ARI) (Agglomerative clustering)

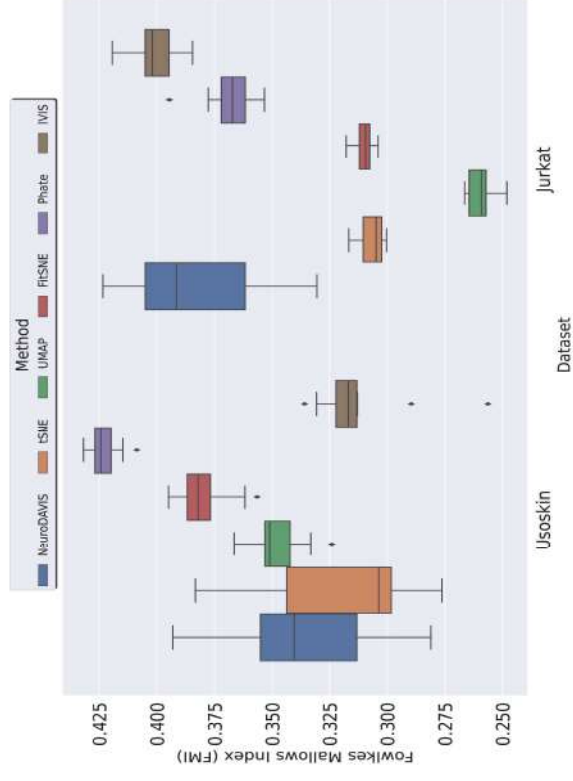

(b) Fowlkes Mallows Index (FMI) (k-means)

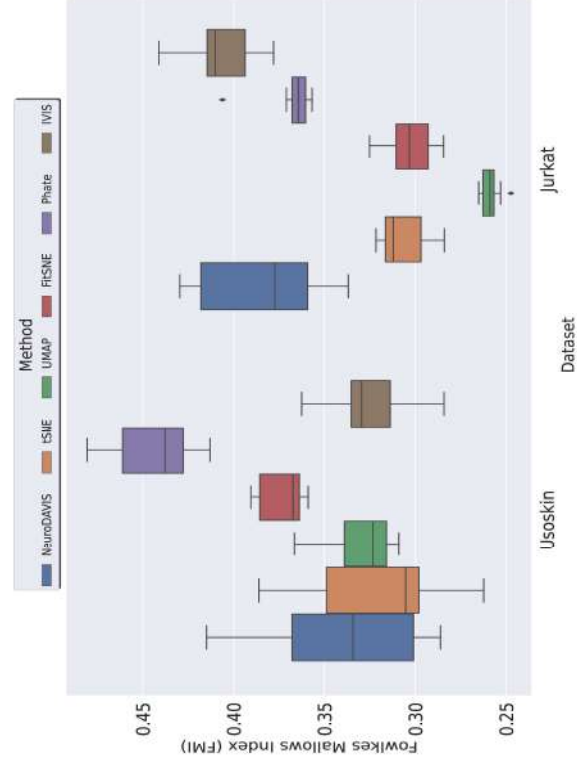

(d) Fowlkes Mallows Index (FMI) (Agglomerative clustering)

**Figure S4:** (a) and (b) show ARI and FMI scores for cell-type clustering using k-means on NeuroDAVIS, t-SNE, UMAP, FIt-SNE, PHATE and IVIS-generated embeddings of Usoskin and Jurkat datasets, (c) (d) show ARI and FMI scores for cell-type clustering using agglomerative hierarchical clustering on NeuroDAVIS, t-SNE, UMAP, FIt-SNE, PHATE and IVIS-generated embeddings of Usoskin and Jurkat datasets.
